# Supplementary material for: SuperNet -- An efficient method of neural networks ensembling
Source: arXiv:2003.13021 source file (2020-03-29)
Supplement: Supplementary file 1 [file appendix.tex]

\chapter*{Appendix A}
